# Supplementary material for: Towards Establishing Dense Correspondence on Multiview Coronary Angiography: From Point-to-Point to Curve-to-Curve Query Matching
Source: arXiv:2312.11593 source file (2023-12-18)
Supplement: Supplementary file 1 [file X_suppl.tex]

\clearpage
\setcounter{page}{1}
\maketitlesupplementary
\begin{table}[h]
  \centering
  \small
   \caption{\textbf{The median and mean distances (in mm) between predicted and ground truth of all relevant points in the testing set, grouped according to their respective projection groups}. For each grid here, the number represents the distances of query points among stenosis markers, bifurcation, and centerline points, given the reference and target groups. The projection groups and their corresponding angles are categorized as follows: A: LAO 40-50°, caudal 25-40°; B: RAO 5-15°, caudal 30°; C: RAO 30-45°, caudal 30-40°; D: RAO 5-10°, cranial 35-40°; E: LAO 30-45°, cranial 25-35°; F: Lateral ±, caudal-cranial 10-30°; G: LAO 45-60°; H: RAO 30-45°. We formatted the table so that smaller numbers are closer to blue color and larger numbers are closer to red color.
   }
  \begin{tabular}{c}
    \begin{minipage}[b]{\linewidth}
		\centering 
		{\includegraphics[width=\linewidth]{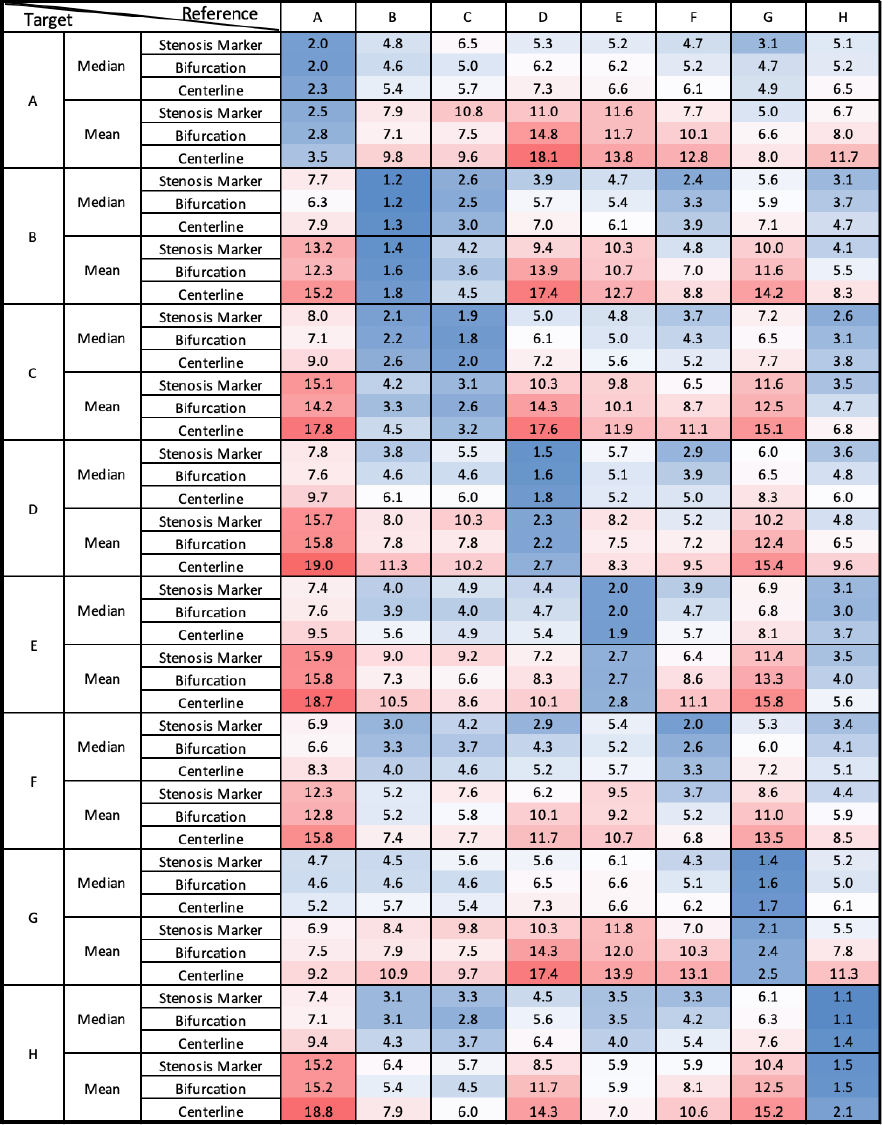}}
	\end{minipage}
  \end{tabular}
  \label{table: result}
\end{table}
